# Supplementary material for: SUSTain: Scalable Unsupervised Scoring for Tensors and its Application to Phenotyping
Source: arXiv:1803.05473 source file (2018-03-14)
Supplement: Supplementary file 1 [file appendix.tex]

\section{Appendix}\label{sec:append}
\noindent \textbf{Proof of Optimal Scaling Lemma~\cite{bro1998least} with integer constraint}

\kimis{Todo add proof of statement:}
\begin{equation*}
{\text{min}} \left\{ || \M{Y} - \V{x}~\V{b}^T ||_2^2 \;\middle|\;
\V{b} \in \mathbb{Z}_{\tau}^N \right\} \Leftrightarrow \Pi_{\mathbb{Z}_{\tau}^N}(\V{\beta})
\end{equation*}
where $\V{\beta} = \frac{\V{x}^T~\M{Y}}{\V{x}^T~\V{x}}$.
